# Supplementary material for: Array oscillator in coupled waveguides with nonlinear gain and radiation resistances saturating at exceptional point
Source: arXiv:2501.14978 source file (2025-02-03)
Supplement: Supplementary file 1 [file Appendix.tex]

\section*{Appendix B: Tolerances analysis of the experimental system}

To ensure the experiment's resilience to tolerances, we consider scenarios where there are variations in the active elements. We examine two different small-signal gains, $g = 4$ and $10$ mS, under two distinct tolerance conditions. Specifically, the gain varies as $g_{n} = 4\times \gamma_{n}$ or $10 \times \gamma_{n}$ mS, where $-5\% < \gamma_{n} < 5\%$ or $-10\% < \gamma_{n} < 10\%$. These variations are illustrated in Fig. \ref{fig:perturbation_measurment}. For the maximum $5\%$ perturbation, the $\gamma_{n}$ values are shown as an inset. Note that the oscillation frequency in all cases is $f_\text{osc} = 124.8$ MHz, and each scenario results in a saturated gain corresponding to a value that leads to an EPD very close to the same frequency.

\begin{figure*}[t]
		\begin{centering}
			\includegraphics[width=7in]{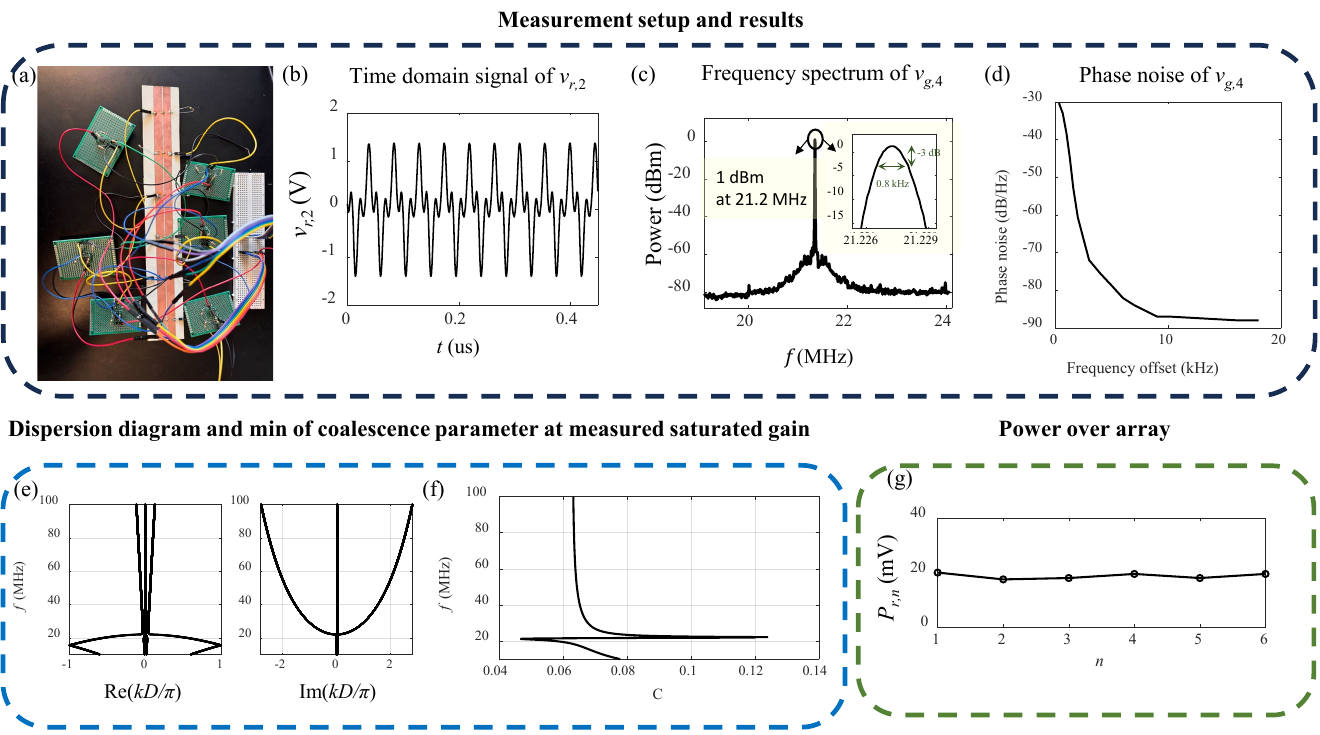}
			\par\end{centering}
		\caption{ Saturated gain of each nonlinear gain element for different small-signal gain values $g=4$ mS and $g=10$ mS with a random perturbation on the array's admittances $-5\%<\gamma_n<5\%$ and  $-10\%<\gamma_n<10\%$ for both small-signal gain values. \label{fig:perturbation_measurment}}
	\end{figure*}

 \section*{Appendix C: Length Analysis of Structures for Power Extraction and Oscillation Frequency Stability}

To ensure the extraction of more power from a longer structure with a stable oscillation frequency, we consider the structure shown in Fig.~(a), which includes a capacitor between the two transmission lines (TLs). We conducted simulations using ADS for structures with $N=9$ to $N=17$ to determine the total power and oscillation frequency. Additionally, we analyze the saturated gain in the middle of the structure as a function of $N$. Our goal is to confirm that the structure operates at the exceptional point of degeneracy for longer configurations.

Figure~(a) illustrates the total power for longer structures, showing a clear increase in power as the structure lengthens. Furthermore, Fig.~(b) demonstrates that the oscillation frequency within the array is $f_\text{osc} = 120.4$ MHz, confirming that the concept of extracting more power from a longer structure with stable oscillation is feasible. Moreover, we present the saturated gain in the middle of the structure as a function of $N$, revealing a smooth slope towards a value of $g_\text{sat} = 2.8$ mS, indicating a second-order exceptional point of degenracy.
